# Supplementary material for: Bounded Verification with On-the-Fly Discrepancy Computation
Source: arXiv:1502.01801 source file (2015-02-06)
Supplement: Supplementary file 1 [file appendix_schur_eigen.tex]

\begin{definition}[Bounds on eigenvalues of Jacobian Matrix]
 We denote the eigenvalues of the symmetric part of the Jacobian by $\lambda_i(\vx,t),~i=1,2,\dots,n$.
%The largest eigenvalue of the Jacobian matrix $\lambda_{max}$ in certain region is the value that satisfies:
%$$\forall \vx \in S, t \in [t_1,t_2], \lambda_{max}\geq \lambda(\vx,t).$$
For a bounded region $S  \subseteq \mathbb{R}^n$ and an interval $[t_1,t_2] \subseteq \mathbb{R}^{\geq 0}$, $\lambda_{max}(S,[t_1,t_2])$ is a real number satisfying
$$
\forall x \in S, t \in [t_1,t_2],\forall i = 1,2,\dots,n,~~\lambda_{max}(S,[t_1,t_2])\geq \lambda_i(\vx,t)
$$
\end{definition}

\begin{theorem}[Symmetric Schur Decomposition]\label{Symmetric Schur Decomposition}
If $A \in \mathbb{R}^{n\times n}$ is symmetric, then there exists a real orthogonal $Q$ such that
$$
Q^T AQ = \Lambda = \mbox{diag}(\lambda _1, \cdots, \lambda _n).
$$
Moreover, for $k=1:n, AQ(:,k)=\lambda _k Q(:,k)$.
\end{theorem}
\begin{proof}
Suppose $\lambda _1 \in \lambda (A)$ and that $x \in \mathbb{C}^n$ is a unit 2-norm eigenvector with $Ax = \lambda _1 x$. Since $\lambda _1 = x ^H Ax = x^H A^H x = \overline{x^H Ax} = \overline{\lambda _1}$ it follows that $\lambda _1 \in \mathbb{R}$. Thus, we may assume that $x \in \mathbb{R}^n$. Let $P_1 \in \mathbb{R}^{n \times n}$ be a Householder matrix such that $P_1^T x = e_1 = I_n(:,1)$. It follows from $Ax = \lambda _1 x $ that $(P_1^T A P _1) e_1 = \lambda e_1$. This says that the first column of $P_1^T A P_1$ is a multiple of $e_1$. But since $P_1^T A P_1$ is symmetric it must have the form
$$P_1^T A P_1 = \left( \begin{array}{cc}
\lambda_1 & 0 \\
0& A_1
\end{array} \right)$$

where $A_1 \in \mathbb{R}^{(n-1) \times (n-1)}$ such that $Q_1^T A_1 Q_1 = \Lambda _1$ is diagonal. The theorem follows by setting
$$
Q = P_1 \left( \begin{array}{cc}
1 & 0 \\
0 & Q_1
\end{array}
\right)
~~~
\mbox{and}
~~~
\Lambda = \left(
\begin{array}{cc}
\lambda _1 & 0 \\
0 & \Lambda_1
\end{array}
\right)
$$
and comparing columns in the matrix equation $AQ = Q\Lambda$
\end{proof}
For a symmetric matrix $A$ we shall use the notation $\lambda _k(A)$ to designate the $k$th largest eigenvalue. Thus,
$$\lambda _n (A) \leq \cdots \leq \lambda _2 (A) \leq \lambda _1 (A)$$

\begin{proposition}\label{Lambda_max}
For any $f:\mathbb{R}^n \times \mathbb{R}^{\geq 0} \rightarrow \mathbb{R}^n$, let $J_{n\times n}(\vx,t)$ be the symmetric part of the Jacobian of $f$.
If $\lambda_{max}(S,[t_1,t_2])$ is the upper bound of eigenvalue of $J_{n\times n}(\vx,t)$ over the region $S,[t_1,t_2]$, then $J(\vx,t)\preceq \lambda_{max}(S,[t_1,t_2])I$, which also implies $\forall \vx \in S, t \in [t_1,t_2],\vy \in \mathbb{R}^n, ~ \vy^T J(\vx,t) \vy \leq \lambda_{max}(S,[t_1,t_2]) \vy^T \vy$
\end{proposition}
\begin{proof}
From theorem \ref{Symmetric Schur Decomposition} we know,$\forall \vx \in S, t \in [t_1,t_2]$,
$J(\vx,t)$ is symmetric, thus $J(\vx,t)$ can be diagnosed as $J(\vx,t) = M^{T}(\vx,t)\Lambda(\vx,t) M(\vx,t)$  where $\Lambda(\vx,t)$ is a diagonal matrix with $\lambda_i(\vx,t),~i=1,2,\dots,n$ and $M(\vx,t)$ is an orthogonal matrix.
Because $\lambda_{max}(\vx,t)\geq \lambda_i(\vx,t), \forall i = 1,2,\dots,n$, we know $\Lambda(\vx,t)-\lambda_{max}(S,[t_1,t_2])I \preceq 0$, furthermore, $M^{T}(\vx,t)(\Lambda(\vx,t)-\lambda_{max}(S,[t_1,t_2])I)M(\vx,t) \preceq 0$,
from which we get $J(\vx,t)-\lambda_{max}(S,[t_1,t_2])I \preceq 0$
\end{proof}

\begin{definition}[Contraction Region]
For any $f:\mathbb{R}^n \times \mathbb{R}^{\geq 0} \rightarrow \mathbb{R}^n$, let $J_{n\times n}(\vx,t)$ be the symmetric part of the Jacobian of $f$.
A region of the state space $S$ is called a contraction region if the symmetric part of Jacobian matrix is uniformly negative definite in that region. By uniformly negative definite we mean that
\begin{equation}\label{uniform contraction}
\exists \beta>0, \forall \vx \in S, \forall t\geq 0,J(\vx,t) = \frac{1}{2}(\frac{\partial f(\vx,t)}{\partial \vx}+\frac{\partial f^{T}(\vx,t)}{\partial \vx})\preceq -\beta I<0
\end{equation}
\end{definition}
